# Supplementary material for: A Setwise Approach for Effective and Highly Efficient Zero-shot Ranking with Large Language Models
Source: arXiv:2310.09497 source file (2024-05-30)
Supplement: Supplementary file 1 [file appendix.tex]

\section{Prompts used in this study}
